# Supplementary material for: Programming-by-Demonstration for Long-Horizon Robot Tasks
Source: arXiv:2305.03129 source file (2023-11-15)
Supplement: Supplementary file 1 [file appendix.tex]

\section{appendix}

\begin{enumerate}
    \item What problem are you working on?
        \begin{itemize} 
          \item We are interested in 
            \item In large open world domains, it is difficult for agents to reason about how to complete tasks. Which objects are relevant? What actions need to be taken on the relevant objects? What order should these actions proceed in?
        \end{itemize}
        
    \item What is the state of the art?
        \begin{itemize}
            \item Give an overview of the general strategies used to solve this problem.
            \begin{itemize}
                \item Using NNs to learn policies over low level actions from NL and video demonstrations.

                \item Should I discuss other methods for synthesis from demonstration that might be relevant here? The first item in this list is relevant to real-world/simulation environments.
            \end{itemize}
        \end{itemize}

        \begin{itemize}
            \item Explain the 2-3 most similar approaches to what you are proposing.
            \begin{itemize}
                \item NN models for solving in simulation
                \begin{itemize}
                    \item Seq2seq model (NNs -- LSTM for sequences of images (encoded with CNNs) alongside NL description to generate low level action sequences \\ https://arxiv.org/pdf/1912.01734.pdf).
                    \item Episodic Transformer (breaks up task into episodes and uses visual sequence of images from episode and actions up to current action, as well as natural language description of task to generate new low level actions. Uses transformers as the NL and action encoders https://arxiv.org/pdf/2105.06453.pdf)
                    \item Soft-Actor Critic and Proximal Policy Optimization as reinforcement learning baselines for Behavior https://arxiv.org/pdf/2108.03332.pdf
                \end{itemize}

                \item Synthesis Methods that are comparable
                \begin{itemize}
                    \item Optimal Neural Program Synthesis from Multimodal Specifications. Uses I/O examples (can think of demonstrations similarly) *and* Natural Language descriptions which we do not require. Also requires dataset to learn model parameters which we do not. https://arxiv.org/pdf/2010.01678.pdf
                    \item Predicting Program Properties from “Big Code”. Trains a model to predict variable types from code examples. Again requires dataset to train model. \\ https://files.sri.inf.ethz.ch/website/papers/jsnice15.pdf
                    \item Accelerating Search-Based Program Synthesis using Learned Probabilistic Models. Uses transfer learning (models learned for other synthesis problems) to probabilistically guide search for programs. Similar, except we are using "transfer learning" to infer information from the natural language meanings in our programs. \\ https://dl.acm.org/doi/pdf/10.1145/3296979.3192410
                    \item Neural Program Synthesis from Diverse Demonstration Videos. Encodes video demonstrations then decodes into programs (uses decoder for actions and perception). Requires large amounts of data (videos of demonstrations and intended output programs). http://proceedings.mlr.press/v80/sun18a/sun18a.pdf
                    \item Language Models as Zero-Shot Planners: Extracting Actionable Knowledge for Embodied Agents. Creates *plans* (not environment agnostic if repetitive like pick up all cups) from large language model queries. https://arxiv.org/pdf/2201.07207.pdf
                    \item WebRobot: Web Robotic Process Automation using Interactive Programming by Demonstration (https://web.eecs.umich.edu/~xwangsd/pubs/pldi22.pdf) and Mimic: Computing Models for Opaque Code (https://stefanheule.com/papers/fse15-mimic.pdf) are two methods for inferring program structure from demonstrations of expected behavior. WebRobot uses human point-click web navigation and Mimic uses program execution to infer source code.
                \end{itemize}
            \end{itemize}
        \end{itemize}

        \begin{itemize} 
            \item What key limitations in the state of the art are you addressing?
            \begin{itemize}
                \item Difficulties in application to large open worlds (many objects, properties, relations and actions). 
                \item Difficulties generalizing to environment instantiations. 
                \item Difficulty with interpretability of solutions (compared to NN solutions).
                \item Better data efficiency compared to NN solutions in large open world environments.
            \end{itemize}
        \end{itemize}

        \begin{itemize} 
            \item What will your approach allow a robot to do that the state of the art does not?
            \begin{itemize} 
                \item Going forward, this method will enable robots to interact in larger open world settings by generating high-level symbolic programs (which act as high-level plans) and then executing these programs with planning over low level actions. This symbolic program will interface with the environment with neural components (e.g. YOLO for object detection). This will reduce the data requirements required to train the current SOTA open world robots.
            \end{itemize}
        \end{itemize}

    \item Why do you believe your approach will overcome the limitations of the state of the art? What technical justification do you have for your approach?
    \begin{itemize}
        \item Symbolically reasoning about open world environments should help improve data efficiency in regards to the total number of training demonstrations, since only a few (possibly one if high quality) symbolic demonstrations are required to solve a task generally.
        \begin{itemize} 
            \item Symbolic program of plan will improve interpretability.
            \item Symbolic program should be environment agnostic which should likely lead to improved generalization to new environments without requiring additional demonstrations.
        \end{itemize}
    \end{itemize}

    \item What evidence will you provide to support that you have succeeded [The answers to all the following should be "yes". If not, you will need to make a convincing argument why not.]
    \begin{itemize}
        \item Are you comparing directly to the state of the art?
            \begin{itemize}
                \item No. Comparing to simulated baselines is not a fair comparison as this paper is only considering symbolic demonstrations and environments. \todo{we cannot simply convince the reader of this. we need a list of closest solutions and explain in more details what are the differences/similarities are between our solution and them, and why we are not reporting any experimental comparisons. This also raises the question "why no one else has looked at your problem? is it even interesting/useful?" which we should be able to answer positively}
                \begin{itemize}
                    \item Not directly comparing with any of the synthesis algorithms as they require datasets that we do not have, or solve problems that are tangential to ours.
                    \item Not comparing with any of the NN solutions as they are in simulation and for the purpose of this paper we are focusing on the synthesis of a high-level program.
                \end{itemize}
            \end{itemize}

        \item Are you using standard benchmarks or existing datasets?
        \begin{itemize}
            \item Somewhat. Adapted tasks from existing benchmarks to be able to apply symbolic solution. \todo{our adaption is minimally affecting the nature of tasks. So I guess we can argue that the benchmarks are standard}
        \end{itemize}

        \item Are you including real-world experiments to show that the approach actually works outside of benchmark data and simulation?
        \begin{itemize}
            \item No. This paper only focuses on the synthesis of symbolic solutions.
        \end{itemize}

        \item Can you prove that your results are correct (e.g. probabilistic completeness for a stochastic planner), or that the claimed performance holds (e.g. time-optimality)?
        \begin{itemize}
            \item Not sure?
            \item \todo {is there any interesting soundness/completeness theorem we can include? -- perhaps in our rewrite and translation rules? I have to think more about this}
        \end{itemize}
    \end{itemize}

    \item What are the limitations of your approach?
    \begin{itemize}
        \item Only symbolic representations considered at the moment.
        \item Synthesis solution relies heavily on the defined open world problem and resultant DSL. \todo {BTW we should be able to defend our DSL and why it is actually general and useful and not crafted for benefiting our experiments in any unjust manner}
    \end{itemize}

    \item What is the single most important point that you want a reader to take away from this paper?
    \begin{itemize}
        \item Symbolic reasoning allows for environment agnostic programs to be synthesized for high level plans to act in large open world environments. 
        \item (Perhaps the use of LLM allows for efficient search for completions -- more relevant to OOPSLA paper).
    \end{itemize}
\end{enumerate}

\begin{itemize}
    \item LfD and why its an important problem and limitations of existing techniques.
    \item Prior work has shown some of the advantages of programmatic LfD but only for reactive controllers, given a sequence of states with their corresponding high-level actions.
    %\item Motivate why you want a programmatic policy and refer to prior work LDIPS to motivate its advantages. LDIPS is intended to synthesize reactive controllers, using labelled human demonstration actions --- in particular, such reactive controllers do not have loops, and arbitrary decision-making criteria. 
    
    \item We want to synthesize robot policies to perform complex tasks that require loops, reasoning about relations and properties of objects, and must operate in large-scale ``open world'' settings that consist of very large numbers of objects, relations, and properties for the synthesizer to reason about.
    \item This problem is challenging for two reasons: First, unlike the reactive controller setting where the shape of the program is fixed a priori, we do not know the actual structure of the programs we want to synthesize. Second, even if we did know the structure, there are too many objects and too many relations between them that the search space the synthesize needs to explore becomes enormous.

    \item In this paper, we propose two key contributions to address the aforementioned issues: 1) we introduce a novel approach to program sketch synthesis from demonstration traces via reduction to RegEx discovery; and 2) we introduce language-model driven program search that exploits the language model's understanding of the most likely relations and properties applied to objects. 
\end{itemize}

Overview of generating partial programs from demonstrations.

\begin{enumerate}
    \item Apply translation rules to produce XML from demonstration.
        \subitem -  Bring hole fills forward if they exist since assumed they will be present in all of appearances within the demonstration.
    \item Use XML schema learner to generate regex of program structure.
    \item Apply rewrite rules recursively on produced regex to get translatable regex.
        \subitem -  (A|B)* -> (AB)*
        \subitem -  (A|B)* -> (AB?)*
        \subitem - \todo{(A|B)* -> (BA)*}
        \subitem - \todo{(A|B)* -> (BA?)*}
        \subitem - \todo{The learner is good at learning the loop structures, but not the contents of the loop. In general, whenever we have a choice of a1|a2|...|an in a loop body, we need to consider all combinations of a1..an with possible conditionals. This will be large for n>2 and we need to find a way to prune the candidate sketches (maybe the infeasiblity check is sufficient to quickly get rid of bad sketches)}
    \item Translate rewritten regex into partial programs.
    \item \todo{we need to start thinking about the formal way of presenting all these concepts. The formalization needs to be precise and concise and at the same time not too low-level. We can discuss it together later. We have list all formal components that we are going to have, e.g., a DSL definition, an operational semantics for it, the syntax of sketches, the translation/rewrite functions or relations, etc.}
\end{enumerate}

\subsection{Partial Program Hole filling}
First attempt to formalize the synthesis:
\begin{itemize}
    \item We are given a partial program $P$
    \subitem -  $P$ has some holes 
    \subitem -  each hole $h$ has a constraint associate to all valid completions of $h$, denoted by $cons(h)$
    \item We have a search algorithm which takes a partial program $P$ and returns a completion of $P^*\in all\_completions\_of(P)$.
    \subitem -  we know some prior knowledge about programs (partial or complete). This probability function is composable and can be applied on each part of the program independently and the overall probability of a programs is defined as multiplication of the probabilities of all of its components. \todo{are we interested in the probability distributions of multi-hole (partial) programs? or is that we only care about distributions over a single hole? -- For now, consider one hole at a time (based on implementation difficulties involving efficient representation of all "legal" pairs of holes e.g. all pairs of object types and properties). }

    \item given a partial program, we want to complete it iteratively. We define a completion path as the sequence of completions from a sketch to a more complete sketch. A path is finalized if the last step fills the last remaining hole. 

    \item at each step on a path, we have to make two decisions
    \subitem -  what should be the next hole to fill?
    \subitem -  what should be the completion to the chosen hole 
 
\end{itemize}

\subsubsection{Search Algorithms} 
Two potential algorithms for searching through potential program completions.

\begin{algorithm}[H]
    Q = {(S, 1)}

    \While{Q $\neq$ 0}{
        (P,$\rho$) = Q.dequeue()\;

        \If{Infeasible(P, D)}{continue}
        \If{Consistent(P, D)}{return P}

        l = SelectLeaf(P)\;
        \For{f $\in$ Supp($M_\theta(\pi$(P,l))}{P' = Fill(P,l,f)\; Q.add((P', $u_\theta$(P'))}
    }
    return None
    \caption{Algorithm from Isil's paper. S is the starting sketch, D is the demo, $M_\theta$ is the language model, and f is a hole fill at the leaf l. $u_\theta$ is a function which uses the the model to produce a ranking for partial programs based on the probability that the partial program is correct (uses a one level look-ahead and the probability of the current path being taken).}
\end{algorithm}

\begin{algorithm}[H]
    l = SelectHole(P)\;

    %F =  Supp($M_\theta$($\pi$(P,l)))\;
    F = GetOrderedHoleFills($M_\theta$, P, l)\;
    %F.sort(by hole fill probability)\ %\todo{we need to start thinking about formal definition of this procedure}\; 

    \For{f $\in$ F}{
        P' = Fill(P,l,f)\;

        \If{Infeasible(P', D)}{continue}
        \If{Consistent(P', D)}{return P'}

        C = recursive call on P' \;

        \If{C $\neq$ None}{
            return C
        }
    }
    return None
    \caption{Recursive Guided depth first search version. S is the starting sketch, D is the demo, $M_\theta$ is the language model, F is the set of hole fills for leaf l, and f is a hole fill at the leaf l.}
\end{algorithm}

\subsubsection{Potential Leaf Orderings}
A few potential methods for picking which hole to fill.

\begin{enumerate}
    \item Pre-order traversal.
    \item Lowest entropy hole fill (hole with high probability prediction for its best fill. E.g. of all hole fills "Cups" for scan(?) has the highest likelihood of being correct -- "Cups" for scan(?) > any hole fill for any other statement)
    \item Hole fill that influences the most other hole fills:
        \subitem -  Most potential hole fills removed across all remaining holes.
        \subitem -  Most other holes are influenced by this hole being filled.
\end{enumerate}

\section{Experiments}

\subsection{Research questions}
\begin{itemize}
    \item How does our approach compare against sota baselines? \begin{itemize}
        \item imitiation learning, using ground truth policy to generate demonstrations
        \item Sergey Levine zero-shot learning 
    \end{itemize}
    What are evaluation metrics (wrt manually written program)?
    \begin{itemize} 
        \item \todo{Plots, metrics/criteria}
        \item Generalization: How many new environments does 
        \item Data efficiency
        \item Robustness: how sensitive is it to changing e
    \end{itemize}
\item How long does it take to learn policies? How sensitive is learning time to number of demos, objects in environment etc
\item How important are two key ideas? Ablation 1: no sketch generation (just search), ablation 2: no guidance with LLM
\end{itemize}
\subsection{Implementation details}
\begin{itemize}
    \item We generate demonstrations either by running ground truth program written by a human for that task and removing some information from them (or) we use an interface for humans to generate these demonstrations in an interactive manner. We assume that some information could be missing from these demos. \todo{how do we generate the missing part?}
\item We use a regex synthesizer to infer the structure from a set of demonstrations
\item We fill the sketch learned so far with the info from demos
For each hole, we fill it with the highest probable value based on a learned neural model
\item The correct program will generate same sequence of action traces as the demonstrations
\item After finding the complete program, we evaluate it against any environment for the same task and show that the goal criteria is met 
\end{itemize}
\subsection{Baselines}
\begin{itemize}
    \item No tools use symbolic demonstrations
    \item \todo{Give  a list of solutions closely related and explain why none of them is a good choice for direct comparison to our solution. Some of this will be used here and some of it in the related works section}
\end{itemize}
\subsection{Dataset}
\begin{itemize}
    \item Hand-curated set of tasks
\item BEHAVIOR - Gibson simulator
\item CHAI - Chalet simulator
\item ALFRED - iTHOR simulator
\item TEACh - AI2-THOR
\item \todo{add a few sentence for each dataset describing it in more details. You can look at how other people have listed/described these datasets in their papers}
\end{itemize}
\subsection{Evaluation criteria}
\begin{itemize}
    \item Accuracy: fraction of solved tasks
    \item Efficiency: number of partial programs searched and run time
\end{itemize}
\subsection{Evaluation}
\todo{we need a table describing our benchmarks, including all variations, etc.}
\begin{itemize}
\item What kind of household tasks do we want to solve?
\begin{itemize}
    \item Supporting State changes and Interaction
    \item Involving intermediate goal conditions
\end{itemize}
\item How does infeasibility pruning affect the number of completions checked and accuracy?
\item How well does our method scale with an increased number of holes?
\begin{itemize}
    \item Perhaps: Easy, Medium, Hard (based on number of holes) 
    \item Perhaps graph based on number of holes vs completion accuracy
\end{itemize}
\item How much does our probability model reduce the number of completions checked and affect accuracy?
\item How well does our algorithm scale to larger environments? \todo{we also need to have a way of classifying environments. Perhaps based on number of rooms and/or number of things in them}
\item How accurate is our method (correct completion set on benchmark)?
\item How well does our method improve with an increased number of demonstrations?
\begin{itemize}
    \item Perhaps: Easy, Medium, Hard (based on number of demos given)
    \item Perhaps graph based on number of demos vs completion accuracy
\end{itemize}
\item Does demonstration source matter? Human vs. From Ground Truth
\item If the user makes a mistake in the demonstration that is noisy – is it correct to be consistent with the demo? Or should we compare with the ground truth \todo{probably should compare to GT, but I am not sure if this reasonable. Must discuss this with profs}
\item How much does the env on which the demo was generated matter
\item How well does a synthesized program generalize to other environments?
\begin{itemize}
    \item Would likely have to compare to the expected ground truth program \todo{yes}
\end{itemize}
\end{itemize}
